# Supplementary material for: Classification As Decoder: Trading Flexibility For Control In Neural Dialogue
Source: arXiv:1910.03476 source file (2019-10-17)
Supplement: Supplementary file 1 [file appendix.tex]

\section{Appendix}
\label{sec:appendix}

\begin{figure}[!htbp]
\begin{center}
\includegraphics[scale=0.2]{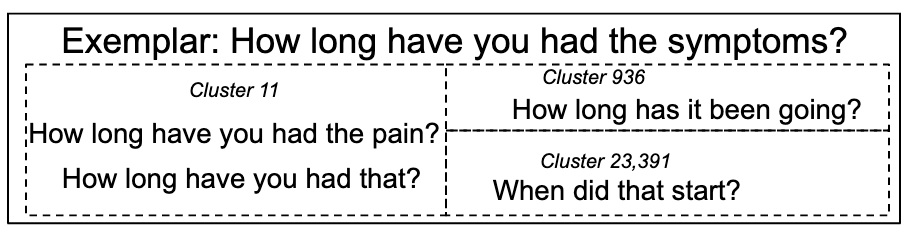}
\caption{Toy example of the components for a response class. The dotted boundaries enclose responses merged in the automatic clustering step, so the two examples in cluster 11 were the only merged responses. The solid boundary encloses the response class. At training time, conversation context preceding all utterances in the box are used as examples of the class. At inference time, if the model predicts this response class, we generate "How long have you had the symptoms", the class exemplar.}
\label{fig:response_gen}
\end{center}
\end{figure}
